# Supplementary material for: Categorical diagonalization and $p$-cells
Source: arXiv:2111.12190 source file (2022-07-05)
Supplement: Supplementary file 1 [file DataTableMoreStatistics.tex]

\begin{tabular}{r | r r | r r r | r r r | r r r | r r | r r r}
Type & $C_2$ & $C_2$ & $G_2$ & $G_2$ & $G_2$ & $C_3$ & $C_3$ & $B_3$ & $C_4$ & $C_4$ & $B_4$ & $D_4$ & $D_4$ & $F_4$ & $F_4$ & $F_4$ \\
$p$ & 0 & 2 & 0 & 2 & 3 & 0 & 2 & 2 & 0 & 2 & 2 & 0 & 2 & 0 & 2 & 3 \\
\hline
\# Left & 4 & 5 & 4 & 6 & 5 & 14 & 17 & 17 & 50 & 63 & 63 & 36 & 38 & 72 & 106 & 78 \\
\# Two-sided & 3 & 4 & 3 & 4 & 4 & 6 & 8 & 8 & 10 & 15 & 15 & 11 & 12 & 11 & 17 & 12 \\
\# $(\mathbf{x}, \pm)$ & 3 & 4 & 3 & 4 & 3 & 6 & 7 & 7 & 9 & 12 & 12 & 7 & 8 & 9 & 12 & 9 \\
\# $\operatorname{Fix} \operatorname{Schu}_L^p$ & 4 & 6 & 4 & 12 & 4 & 32 & 40 & 40 & 280 & 332 & 332 & 112 & 120 & 544 & 1136 & 544 \\
\# $\operatorname{Unfix} \operatorname{Schu}_L^p$ & 4 & 2 & 8 & 0 & 8 & 16 & 8 & 8 & 104 & 52 & 52 & 80 & 72 & 608 & 16 & 608 \\
\end{tabular}
